# Supplementary material for: REAL Sampling: Boosting Factuality and Diversity of Open-Ended Generation via Asymptotic Entropy
Source: arXiv:2406.07735 source file (2024-06-11)
Supplement: Supplementary file 1 [file old_C_visualization.tex]

% \begin{figure}[t!]
% \centering
% \includegraphics[width=1\linewidth]{figs/visualization.pdf}
% \caption{The visualization of the estimated residual entropy ($\hat{d}_c^{RE}$) for the first twelve testing factual prompts in \textsc{FactualityPrompts} and their generated continuations. More yellow means a larger next-token hallucination likelihood from our THF model and thus a smaller $p$ threshold in REAL sampling.}
% %\mbc{nice fig! but `real lm' is sounding like it's a real vs./ unreal LM? so we should change REAL to a slightly different acronym? also highlight the red and green arrows coming from the left to right a bit bolder/thicker}} 
% \label{fig:visualization}
% \end{figure}

% \section{Qualitative Analysis}
% \label{sec:visualization}
% %In \Cref{fig:comp_gen_entail}, 

% We visualize the residual entropy (RE) from our THF model in \Cref{fig:visualization}. As we illustrated in \Cref{fig:asymptotic_entropy}, the residual entropy tends to be larger when the next token is very likely to be an entity while tends to be small near the beginning of the sentence. For example, in the left-most example, the token before the \textit{Hollywood} received the highest RE in the sequence. Nevertheless, the non-entity next token could also receive a high RE. Taking the second from right sequence as an example, the next token of \textit{Walt Disney has a} has a high RE but the chance of having an entity after the token \textit{a} is not very high and the ground truth token \textit{brother} is indeed not an entity.
